# Supplementary material for: Impact of magnetic anisotropy on the magnon Hanle effect in $\alpha$-Fe$_2$O$_3$
Source: arXiv:2306.00375 source file (2023-06-01)
Supplement: Supplementary file 1 [file Supplementary_material.pdf]

# Supplemental Material: Impact of magnetic anisotropy on the magnon Hanle effect in $\alpha$-$Fe_2O_3$

M. Scheufele,[1,2,a)] J. Gückelhorn,[1,2] M. Opel,[1] A. Kamra,[3] H. Huebl,[1,2,4] R. Gross,[1,2,4] S. Geprägs,[1] and M. Althammer[1,2,b)]

[1)] *Walther-Meißner-Institut, Bayerische Akademie der Wissenschaften, 85748 Garching, Germany*

[2)] *Technische Universität München, TUM School of Natural Sciences, Physics Department, 85748 Garching, Germany*

[3)] *Condensed Matter Physics Center (IFIMAC) and Departamento de Física Teórica de la Materia Condensada, Universidad Autónoma de Madrid, 28049 Madrid, Spain*

[4)] *Munich Center for Quantum Science and Technology (MCQST), 80799 Munich, Germany*

(Dated: 1 June 2023)

[a)] Author to whom correspondence should be addressed: monika.scheufele@wmi.badw.de

[b)] Electronic mail: matthias.althammer@wmi.badw.de

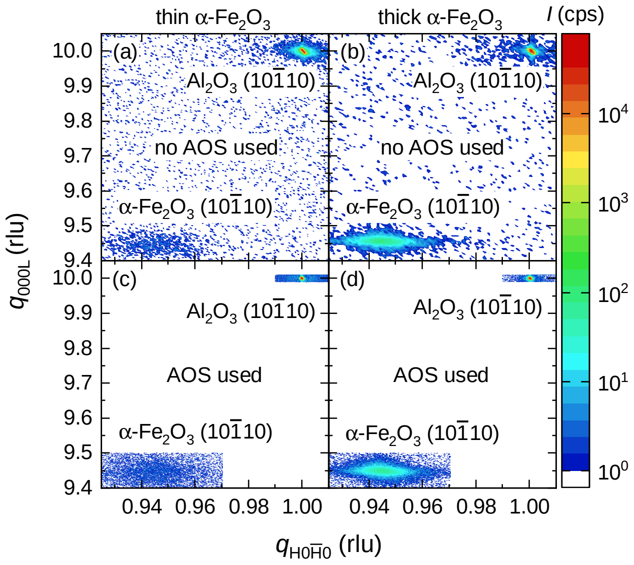


FIG. S1. Reciprocal space mapping around the $(10\bar{1}\,10)$ reflection of a (a) 25 nm, (b) 124 nm, (c) 19 nm and (d) 89 nm thick $\alpha$-$Fe_2O_3$ film. The units are given in reciprocal lattice units (rlu) with respect to the $Al_2O_3$ $(10\bar{1}\,10)$ substrate reflections. The upper (lower) panels represent $\alpha$-$Fe_2O_3$ films grown without (with) the addition of atomic oxygen during the deposition process.

## I. CRYSTALLOGRAPHIC PROPERTIES OF HEMATITE FILMS

The $\alpha$-$Fe_2O_3$ films discussed in this article are grown on hexagonal (0001)-oriented $Al_2O_3$ substrates, which results in a large lattice mismatch $\varepsilon = (a_{\alpha-\mathrm{Fe_2O_3,bulk}} - a_{\mathrm{Al_2O_3}})/a_{\mathrm{Al_2O_3}}$ of 5.8 %[1,2]. Therefore, we expect a fully relaxed growth of $\alpha$-$Fe_2O_3$ on $Al_2O_3$ (0001).

To analyze the strain state of the $\alpha$-$Fe_2O_3$ films, we perform reciprocal space mappings (RSMs) around the asymmetric $\alpha$-$Fe_2O_3$ $(10\bar{1}\,10)$ and $Al_2O_3$ $(10\bar{1}\,10)$ reflections as shown in Fig. S1 for (a), (c) thin and (b), (d) thick $\alpha$-$Fe_2O_3$ films grown without [(a) and (b)] and with [(c) and (d)] atomic oxygen. The RSMs and the $2\theta$-$\omega$ scans in Fig. 1 (a) and (b) in the main text confirm the epitaxial relations $\alpha$-$Fe_2O_3$ [0001] $\|$ $Al_2O_3$ [0001] and $\alpha$-$Fe_2O_3$ $[10\bar{1}0]$ $\|$ $Al_2O_3$ $[10\bar{1}0]$ between the respective film and substrate.

We extract the $\alpha$-$Fe_2O_3$ and $Al_2O_3$ reflection positions given by $q_{\mathrm{H0\bar{H}0}}$ and $q_{\mathrm{000L}}$ in Fig. S1 and calculate the in-plane and out-of-plane lattice constants $a_{\mathrm{RSM}}$ and $c_{\mathrm{RSM}}$ of $\alpha$-$Fe_2O_3$. Together with $c_{2\theta-\omega}$ extracted from the corresponding $2\theta$-$\omega$ scans, we derive the average $c = (c_{2\theta-\omega} + c_{\mathrm{RSM}})/2$ and display $a = a_{\mathrm{RSM}}$ and $c$ in Fig. S2 as a function of the $\alpha$-$Fe_2O_3$ film thickness $t_{\mathrm{m}}$. Since the reflections in Fig. S1 are fitted to Gaussian functions, the error of $a$ is determined by the fit

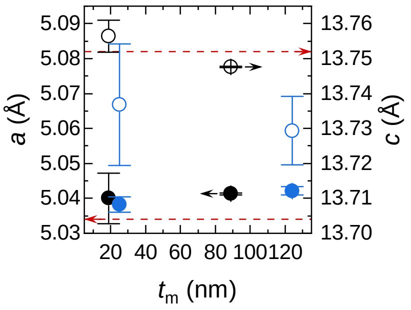


FIG. S2. In-plane lattice constant $a$ (full circles) and out-of-plane lattice constant $c$ (open circles) as functions of the $\alpha$-$Fe_2O_3$ film thickness $t_m$. Black and blue symbols indicate films grown with and without atomic oxygen, respectively. The red dashed lines refer to the bulk values of $\alpha$-$Fe_2O_3$ of $a = 5.034\,\text{Å}$ and $c = 13.752\,\text{Å}$[1].

errors and corresponding error propagation. The error of the mean value $c$ is simply given by the standard deviation. The thus obtained lattice constants $a$ are nearly constant over the whole thickness range and close to the bulk value of $a = 5.034\,\text{Å}$[1]. The epitaxial in-plane strain $\varepsilon_{xx} = (a - a_{\alpha-Fe_2O_3,bulk})/a_{\alpha-Fe_2O_3,bulk}$ is in the range of $0.08(4)\,\% - 0.16(2)\,\%$ for all $\alpha$-$Fe_2O_3$ films investigated. Furthermore, we do not observe a dependence of $\varepsilon_{xx}$ on whether the $\alpha$-$Fe_2O_3$ films are grown with atomic oxygen or not. Therefore, the small $\varepsilon_{xx}$ suggests a nearly relaxed growth of $\alpha$-$Fe_2O_3$ on $Al_2O_3$ (0001) for all investigated $\alpha$-$Fe_2O_3$ films. We observe a slight increase in $c$ for the $\alpha$-$Fe_2O_3$ films grown with atomic oxygen compared to films fabricated without atomic oxygen, which is more pronounced for the thicker $\alpha$-$Fe_2O_3$ films.

## II. ALL-ELECTRICAL MAGNON TRANSPORT MEASUREMENTS

### A. Technical details

For all-electrical magnon transport experiments, we first pattern two-strip structures with different center-to-center distances $d$ on top of the $\alpha$-$Fe_2O_3$ films via electron beam lithography and deposit *ex-situ* polycrystalline Pt of 5 nm thickness via DC magnetron sputtering and a subsequent lift-off process. Both Pt strips are 500 nm wide and 100 µm long. Secondly, we pattern 50 nm thick Al leads and bond pads to allow for an electrical injection and detection of magnons.

Using a Keithley 2400 current source, we apply a DC charge current $I_{inj} = 500\,\mu A$ to one Pt electrode inducing a $z$-polarized electron spin accumulation at the $\alpha$-$Fe_2O_3$/Pt interface via

the spin Hall effect (SHE, see coordinate system in Fig. 2 (a) in the main text)[3–5]. At finite temperatures, this leads to an excitation of magnons in the $\alpha$-$Fe_2O_3$ film, if the Néel order parameter $\boldsymbol{n}$ is not perpendicular to the spin polarization $\boldsymbol{s}$. The magnons then propagate diffusively in the $\alpha$-$Fe_2O_3$ film towards the second Pt electrode. Meanwhile, the pseudospin of the magnons precesses around the pseudofield $\boldsymbol{\omega}$, since the injected, circular-polarized magnons are not the eigenexcitations of a magnetically easy-plane antiferromagnet[6,7]. At the second Pt electrode, the $z$-component of the magnon pseudospin is electrically detected as the voltage signal $V_{\mathrm{det}}$ with a Keithley 2182 nanovoltmeter via the inverse SHE (iSHE)[4,8]. To eliminate signals from thermally induced magnons, we use the current reversal technique to get the voltage signal $V_{\mathrm{det}}^{\mathrm{el}} = [V_{\mathrm{det}}(+I_{\mathrm{inj}}) - V_{\mathrm{det}}(-I_{\mathrm{inj}})]/2$ stemming from electrically excited magnons[9,10].

## B. Fit parameters of the thin $\alpha$-$Fe_2O_3$ films

We fit the magnon Hanle curves of the thin $\alpha$-$Fe_2O_3$ films depicted in Fig. 2 (b) and (d) and Fig. 3 (a) and (c) in the main text to

$$\Delta R_{\mathrm{det}}^{\mathrm{el}} = \Delta R_{\mathrm{det},0}^{\mathrm{el}} + \frac{A l_{\mathrm{m}} e^{-\frac{ad}{l_{\mathrm{m}}}}}{D_{\mathrm{m}}(a^2+b^2)} \left( a \cos\left(\frac{bd}{l_{\mathrm{m}}}\right) - b \sin\left(\frac{bd}{l_{\mathrm{m}}}\right) \right) \tag{S1}$$

with the finite offset $\Delta R_{\mathrm{det},0}^{\mathrm{el}}$, the amplitude $A = A_0 j_{\mathrm{s}0}/\chi$, the magnon spin decay length $l_{\mathrm{m}} = \sqrt{D_{\mathrm{m}} \tau_{\mathrm{m}}}$ and $a, b = \sqrt{(\sqrt{1+\omega^2\tau_{\mathrm{m}}^2} \pm 1)/2}$. $A_0$ is a constant scaling parameter, $j_{\mathrm{s}0}$ is the magnon spin current density driven by the injector, $\chi$ is the susceptibility relating the pseudospin density to the pseudospin chemical potential, $D_{\mathrm{m}}$ is the magnon diffusion constant and $\tau_{\mathrm{m}}$ is the magnon spin relaxation time[6]. We treat the pseudofield as an experimentally observed field and perform a Taylor expansion of the precession frequency $\omega$ around the compensation field $H_{\mathrm{c}}$ leading to $\omega = -c_1 + c_2 H$. The extracted free fit parameters $\Delta R_{\mathrm{det},0}^{\mathrm{el}}$, $A$, $D_{\mathrm{m}}$, $\tau_{\mathrm{m}}$, $c_1$ and $c_2$ of the fits in Fig. 2 (b) and (d) in the main text are given in Table S1. The injector-detector distance $d$ is hereby a fixed fit parameter.

The maximum amplitude of the electrically induced magnon spin signal is determined by $\Delta R_{\mathrm{det}}^{\mathrm{el}}(\mu_0 H_{\mathrm{c}}) = \Delta R_{\mathrm{det},0}^{\mathrm{el}} + A l_{\mathrm{m}} \exp(-d/l_{\mathrm{m}})/D_{\mathrm{m}}$, as $\omega$ is zero at the compensation field. Comparing the fit parameters of devices on $\alpha$-$Fe_2O_3$ films fabricated with (AOS-$Fe_2O_3$) and without (NAOS-$Fe_2O_3$) atomic oxygen for $d = 750\,\mathrm{nm}$ and $d = 700\,\mathrm{nm}$, respectively, we can conclude that the larger magnon Hanle signal at the compensation field for the AOS-$Fe_2O_3$ film is caused by a larger magnon spin decay length. In case of devices with $d = 1000\,\mathrm{nm}$, the AOS-$Fe_2O_3$ film ex-

TABLE S1. Extracted parameters from the fits to Eq. (S1) in Fig. 2 (b), (d) in the main text. The thickness of the NAOS-$Fe_2O_3$ and the AOS-$Fe_2O_3$ film is 15 nm and 19 nm, respectively. The calculated magnon spin decay length $l_m$ and maximum amplitude $\Delta R^{el}_{det}(\mu_0 H_c)$ of the electrically induced magnon spin signal are presented as well.

| Symbol | Unit | NAOS-$Fe_2O_3$ | NAOS-$Fe_2O_3$ | AOS-$Fe_2O_3$ | AOS-$Fe_2O_3$ |
|---|---|---|---|---|---|
| $d$ | nm | 700 | 1000 | 750 | 1000 |
| $\Delta R^{el}_{det,0}$ | mΩ | $0.16 \pm 0.01$ | $0.019 \pm 0.002$ | $0.11 \pm 0.01$ | $-0.04 \pm 0.01$ |
| $A$ | $\Omega\,m\,s^{-1}$ | $4.4 \pm 4.9$ | $0.7 \pm 0.2$ | $2.6 \pm 0.5$ | $4.6 \pm 5.3$ |
| $D_m$ | $10^{-4} m^2\,s^{-1}$ | $1.0 \pm 0.6$ | $2.6 \pm 0.9$ | $2.5 \pm 1.2$ | $1.7 \pm 1.2$ |
| $\tau_m$ | ns | $0.5 \pm 0.5$ | $0.1 \pm 0.2$ | $0.8 \pm 0.2$ | $0.6 \pm 0.3$ |
| $c_1$ | $10^9 s^{-1}$ | $-7.7 \pm 4.9$ | $9.6 \pm 1.9$ | $12.3 \pm 3.6$ | $15.8 \pm 5.7$ |
| $c_2$ | $10^9 m/(As)$ | $-1.0 \pm 0.6$ | $1.2 \pm 0.3$ | $1.6 \pm 0.5$ | $2.2 \pm 0.8$ |
| $l_m$ | nm | $223 \pm 69$ | $510 \pm 89$ | $447 \pm 108$ | $319 \pm 113$ |
| $\Delta R^{el}_{det}(\mu_0 H_c)$ | mΩ | $0.59 \pm 0.78$ | $0.21 \pm 0.07$ | $0.98 \pm 0.24$ | $0.34 \pm 0.58$ |

hibits a larger amplitude $A$ resulting in a larger $\Delta R^{el}_{det}(\mu_0 H_c)$. Therefore, the larger magnon Hanle signal at $\mu_0 H_c$ for the AOS-$Fe_2O_3$ films can be explained by an increase in $A \propto j_{s0}/\chi$ and $l_m$, respectively.

Additional measurements of the spin Hall magnetoresistance (SMR) reveal similar SMR amplitudes between $3 \times 10^{-4}$ and $7 \times 10^{-4}$ for all investigated $\alpha$-$Fe_2O_3$ films. This proves that the spin transparency between the Pt strips and the $\alpha$-$Fe_2O_3$ films is nearly constant and not dependent on the fabrication process of the $\alpha$-$Fe_2O_3$ films. Therefore, the increase in the factor $A$ is not due to an increase in $j_{s0}$, but due to a decrease in $\chi$.

## C. Temperature dependence of the amplitude of the electrically induced magnon spin signal at the compensation field

In the following, we complement the data presented in Fig. 4 (c) and (d) in the main part. Therefore, Fig. S3 depicts the maximum amplitude $\Delta R^{el}_{det}$ of the electrically induced magnon spin signal extracted at the compensation field $\mu_0 H_c$ as a function of temperature $T$ for different injector-detector distances $d$. We categorize in (a) thin and (b) thick films and in NAOS-$Fe_2O_3$ (blue

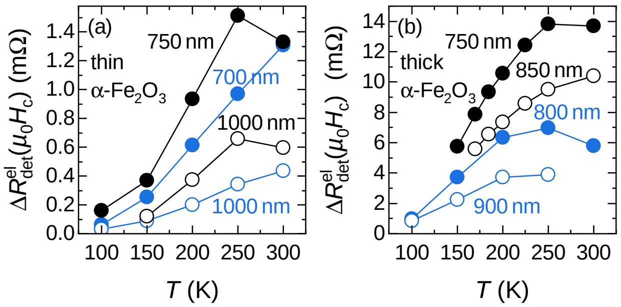


FIG. S3. Maximum amplitude $\Delta R^{\mathrm{el}}_{\mathrm{det}}$ of the electrically induced magnon spin signal extracted at the compensation field $\mu_0 H_{\mathrm{c}}$ as a function of temperature $T$. The center-to-center distances between injector and detector range from 700 nm to 1000 nm depending on the investigated $\alpha$-$Fe_2O_3$ film. The thickness of the NAOS-$Fe_2O_3$ films (blue circles) are (a) 15 nm and (b) 103 nm, whereas the AOS-$Fe_2O_3$ films (black circles) are (a) 19 nm and (b) 89 nm thick.

circles) and AOS-$Fe_2O_3$ films (black circles). For all four $\alpha$-$Fe_2O_3$ films, we observe a decrease in $\Delta R^{\mathrm{el}}_{\mathrm{det}}(\mu_0 H_{\mathrm{c}})$, when increasing $d$. Additionally, the peak-like behavior of $\Delta R^{\mathrm{el}}_{\mathrm{det}}(\mu_0 H_{\mathrm{c}})$ for the AOS-$Fe_2O_3$ film in (a) and both $\alpha$-$Fe_2O_3$ films in (b) is also visible for larger $d$.

### D. Determination of the magnon spin decay length in thick hematite films

Since the contribution of low-energy magnons in thick $\alpha$-$Fe_2O_3$ films leads to a finite offset in $\Delta R^{\mathrm{el}}_{\mathrm{det}}$ at low magnetic fields, appropriate fitting of the Hanle peak to Eq. (1) in the main part is challenging. Therefore, magnon transport parameters such as the magnon spin decay length $l_{\mathrm{m}}$ need to be determined in a different manner. We demonstrate the corresponding procedure exemplary for the 103 nm thick $\alpha$-$Fe_2O_3$ film grown without the addition of atomic oxygen. We first extract $\Delta R^{\mathrm{el}}_{\mathrm{det}}$ at a constant magnetic field magnitude of 2 T for temperatures $50\,\mathrm{K} \leq T \leq 300\,\mathrm{K}$ (cf. Fig. 3 (b) of the main part). Fig. S4 (a) presents the results for several injector-detector distances $d$ ranging from 550 nm to 900 nm. $\Delta R^{\mathrm{el}}_{\mathrm{det}}$ increases with increasing $T$ and then decreases for temperatures above 200 K except for $d = 550\,\mathrm{nm}$, where $\Delta R^{\mathrm{el}}_{\mathrm{det}}$ further increases. With increasing $T$ the thermal population of magnon states in $\alpha$-$Fe_2O_3$ increases. However, at sufficiently high temperatures magnon scattering reduces $l_{\mathrm{m}}$ and thus $\Delta R^{\mathrm{el}}_{\mathrm{det}}$ decreases again. At constant temperature, we can plot $\Delta R^{\mathrm{el}}_{\mathrm{det}}$ as function of $d$ for different $T$ and observe an exponential decay of $\Delta R^{\mathrm{el}}_{\mathrm{det}}(d)$ as

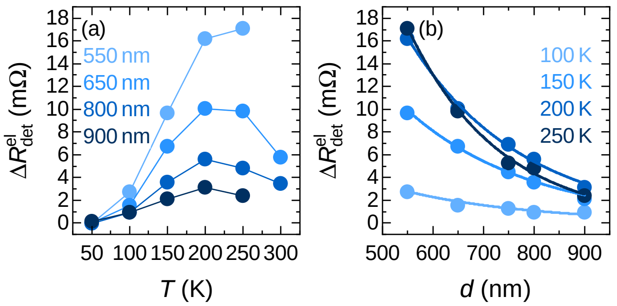


FIG. S4. Amplitude $\Delta R_{\mathrm{det}}^{\mathrm{el}}$ of the electrically induced magnon spin signal of the 103 nm thick NAOS-$Fe_2O_3$ film at a magnetic field magnitude of 2 T. (a) $\Delta R_{\mathrm{det}}^{\mathrm{el}}$ as a function of temperature $T$ for different center-to-center distances $d$ between injector and detector. The solid lines are guides to the eye. Fixing the temperature, we can extract $\Delta R_{\mathrm{det}}^{\mathrm{el}}$ as a function of $d$ as shown in (b). The solid lines are fits to Eq. (S2).

shown in Fig. S4 (b). The solid lines are fits to[11]

$$\Delta R_{\mathrm{det}}^{\mathrm{el}} = \frac{C}{l_{\mathrm{m}}} \frac{\exp\left(d/l_{\mathrm{m}}\right)}{1-\exp\left(2d/l_{\mathrm{m}}\right)}, \tag{S2}$$

with the constant prefactor $C$. This allows us to extract $l_{\mathrm{m}}$ given in Fig. 4 (f) in the main part. The behavior of $\Delta R_{\mathrm{det}}^{\mathrm{el}}$ as a function of $T$ as well as of $d$ is in agreement with previous literature[12].

## REFERENCES

[1] "$\alpha$-$Fe_2O_3$ hematite ($Fe_2O_3$ hem) Crystal Structure: Datasheet from "PAULING FILE Multinaries Edition – 2022" in SpringerMaterials," Copyright 2016 Springer-Verlag Berlin Heidelberg & Material Phases Data System (MPDS), Switzerland & National Institute for Materials Science (NIMS), Japan.

[2] "$Al_2O_3$ Crystal Structure: Datasheet from "PAULING FILE Multinaries Edition – 2022" in SpringerMaterials," Copyright 2016 Springer-Verlag Berlin Heidelberg & Material Phases Data System (MPDS), Switzerland & National Institute for Materials Science (NIMS), Japan.

[3] J. E. Hirsch, "Spin Hall Effect," Phys. Rev. Lett. **83**, 1834–1837 (1999).

[4] J. Sinova, S. O. Valenzuela, J. Wunderlich, C. H. Back, and T. Jungwirth, "Spin Hall effects," Rev. Mod. Phys. **87**, 1213–1260 (2015).

[5] R. Lebrun, A. Ross, S. A. Bender, A. Qaiumzadeh, L. Baldrati, J. Cramer, A. Brataas, R. A. Duine, and M. Kläui, "Tunable long-distance spin transport in a crystalline antiferromagnetic iron oxide," Nature **561**, 222–225 (2018).

[6]A. Kamra, T. Wimmer, H. Huebl, and M. Althammer, "Antiferromagnetic magnon pseudospin: Dynamics and diffusive transport," Phys. Rev. B **102**, 174445 (2020).

[7]T. Wimmer, A. Kamra, J. Gückelhorn, M. Opel, S. Geprägs, R. Gross, H. Huebl, and M. Althammer, "Observation of Antiferromagnetic Magnon Pseudospin Dynamics and the Hanle Effect," Phys. Rev. Lett. **125**, 247204 (2020).

[8]E. Saitoh, M. Ueda, H. Miyajima, and G. Tatara, "Conversion of spin current into charge current at room temperature: Inverse spin-Hall effect," Appl. Phys. Lett. **88**, 182509 (2006).

[9]S. T. B. Goennenwein, R. Schlitz, M. Pernpeintner, K. Ganzhorn, M. Althammer, R. Gross, and H. Huebl, "Non-local magnetoresistance in YIG/Pt nanostructures," Appl. Phys. Lett. **107**, 172405 (2015).

[10]K. Ganzhorn, S. Klingler, T. Wimmer, S. Geprägs, R. Gross, H. Huebl, and S. T. B. Goennenwein, "Magnon-based logic in a multi-terminal YIG/Pt nanostructure," Appl. Phys. Lett. **109**, 022405 (2016).

[11]L. J. Cornelissen, J. Liu, R. A. Duine, J. B. Youssef, and B. J. V. Wees, "Long-distance transport of magnon spin information in a magnetic insulator at room temperature," Nat. Phys. **11**, 1022–1026 (2015).

[12]J. Han, P. Zhang, Z. Bi, Y. Fan, T. S. Safi, J. Xiang, J. Finley, L. Fu, R. Cheng, and L. Liu, "Birefringence-like spin transport via linearly polarized antiferromagnetic magnons," Nat. Nanotechnol. **15**, 563–568 (2020).
